# Supplementary material for: BEVHeight++: Toward Robust Visual Centric 3D Object Detection
Source: arXiv:2309.16179 source file (2023-09-28)
Supplement: Supplementary file 1 [file 5-appendix-arxiv.tex]

\section{Appendix}

\subsection{Broader Impacts} % \Tao{repeats with limitation?}
Our work aims to develop a vision-based 3D object detection approach for roadside perception. The proposed method may produce inaccurate predictions, leading to incorrect decision-making for cooperative autonomous vehicles and potential traffic accidents. Furthermore, we propose a new perspective of leveraging height estimation to solve PV-BEV transformation, facilitating a high-performance and robust vision-centric BEV perception framework. Although considerable progress has been made with our proposed height net and height-based 2D-3D projection module, we believe it is worth further exploring how to combine height and depth estimations to extend to autonomous driving scenarios.

\subsection{Dynamic Discretization}
The height discretization can be performed with uniform discretization (UD) with a fixed bin size, spacing-increasing discretization (SID)~\cite{HuanFu2018DeepOR} with increasing bin sizes in logspace, linear-increasing discretization (LID)~\cite{YunleiTang2020Center3DCM}and our proposed dynamic-increasing discretization (DID) with adjustable bin sizes. The above four height discretization techniques are visualized in Fig. \ref{fig:discretization}. Following DID strategy, the distribution of height bins can be dynamically adjusted with different hyper-parameter $\alpha$.

%figure7
\begin{figure}[ht]
\centering	\includegraphics[width=8.5cm]{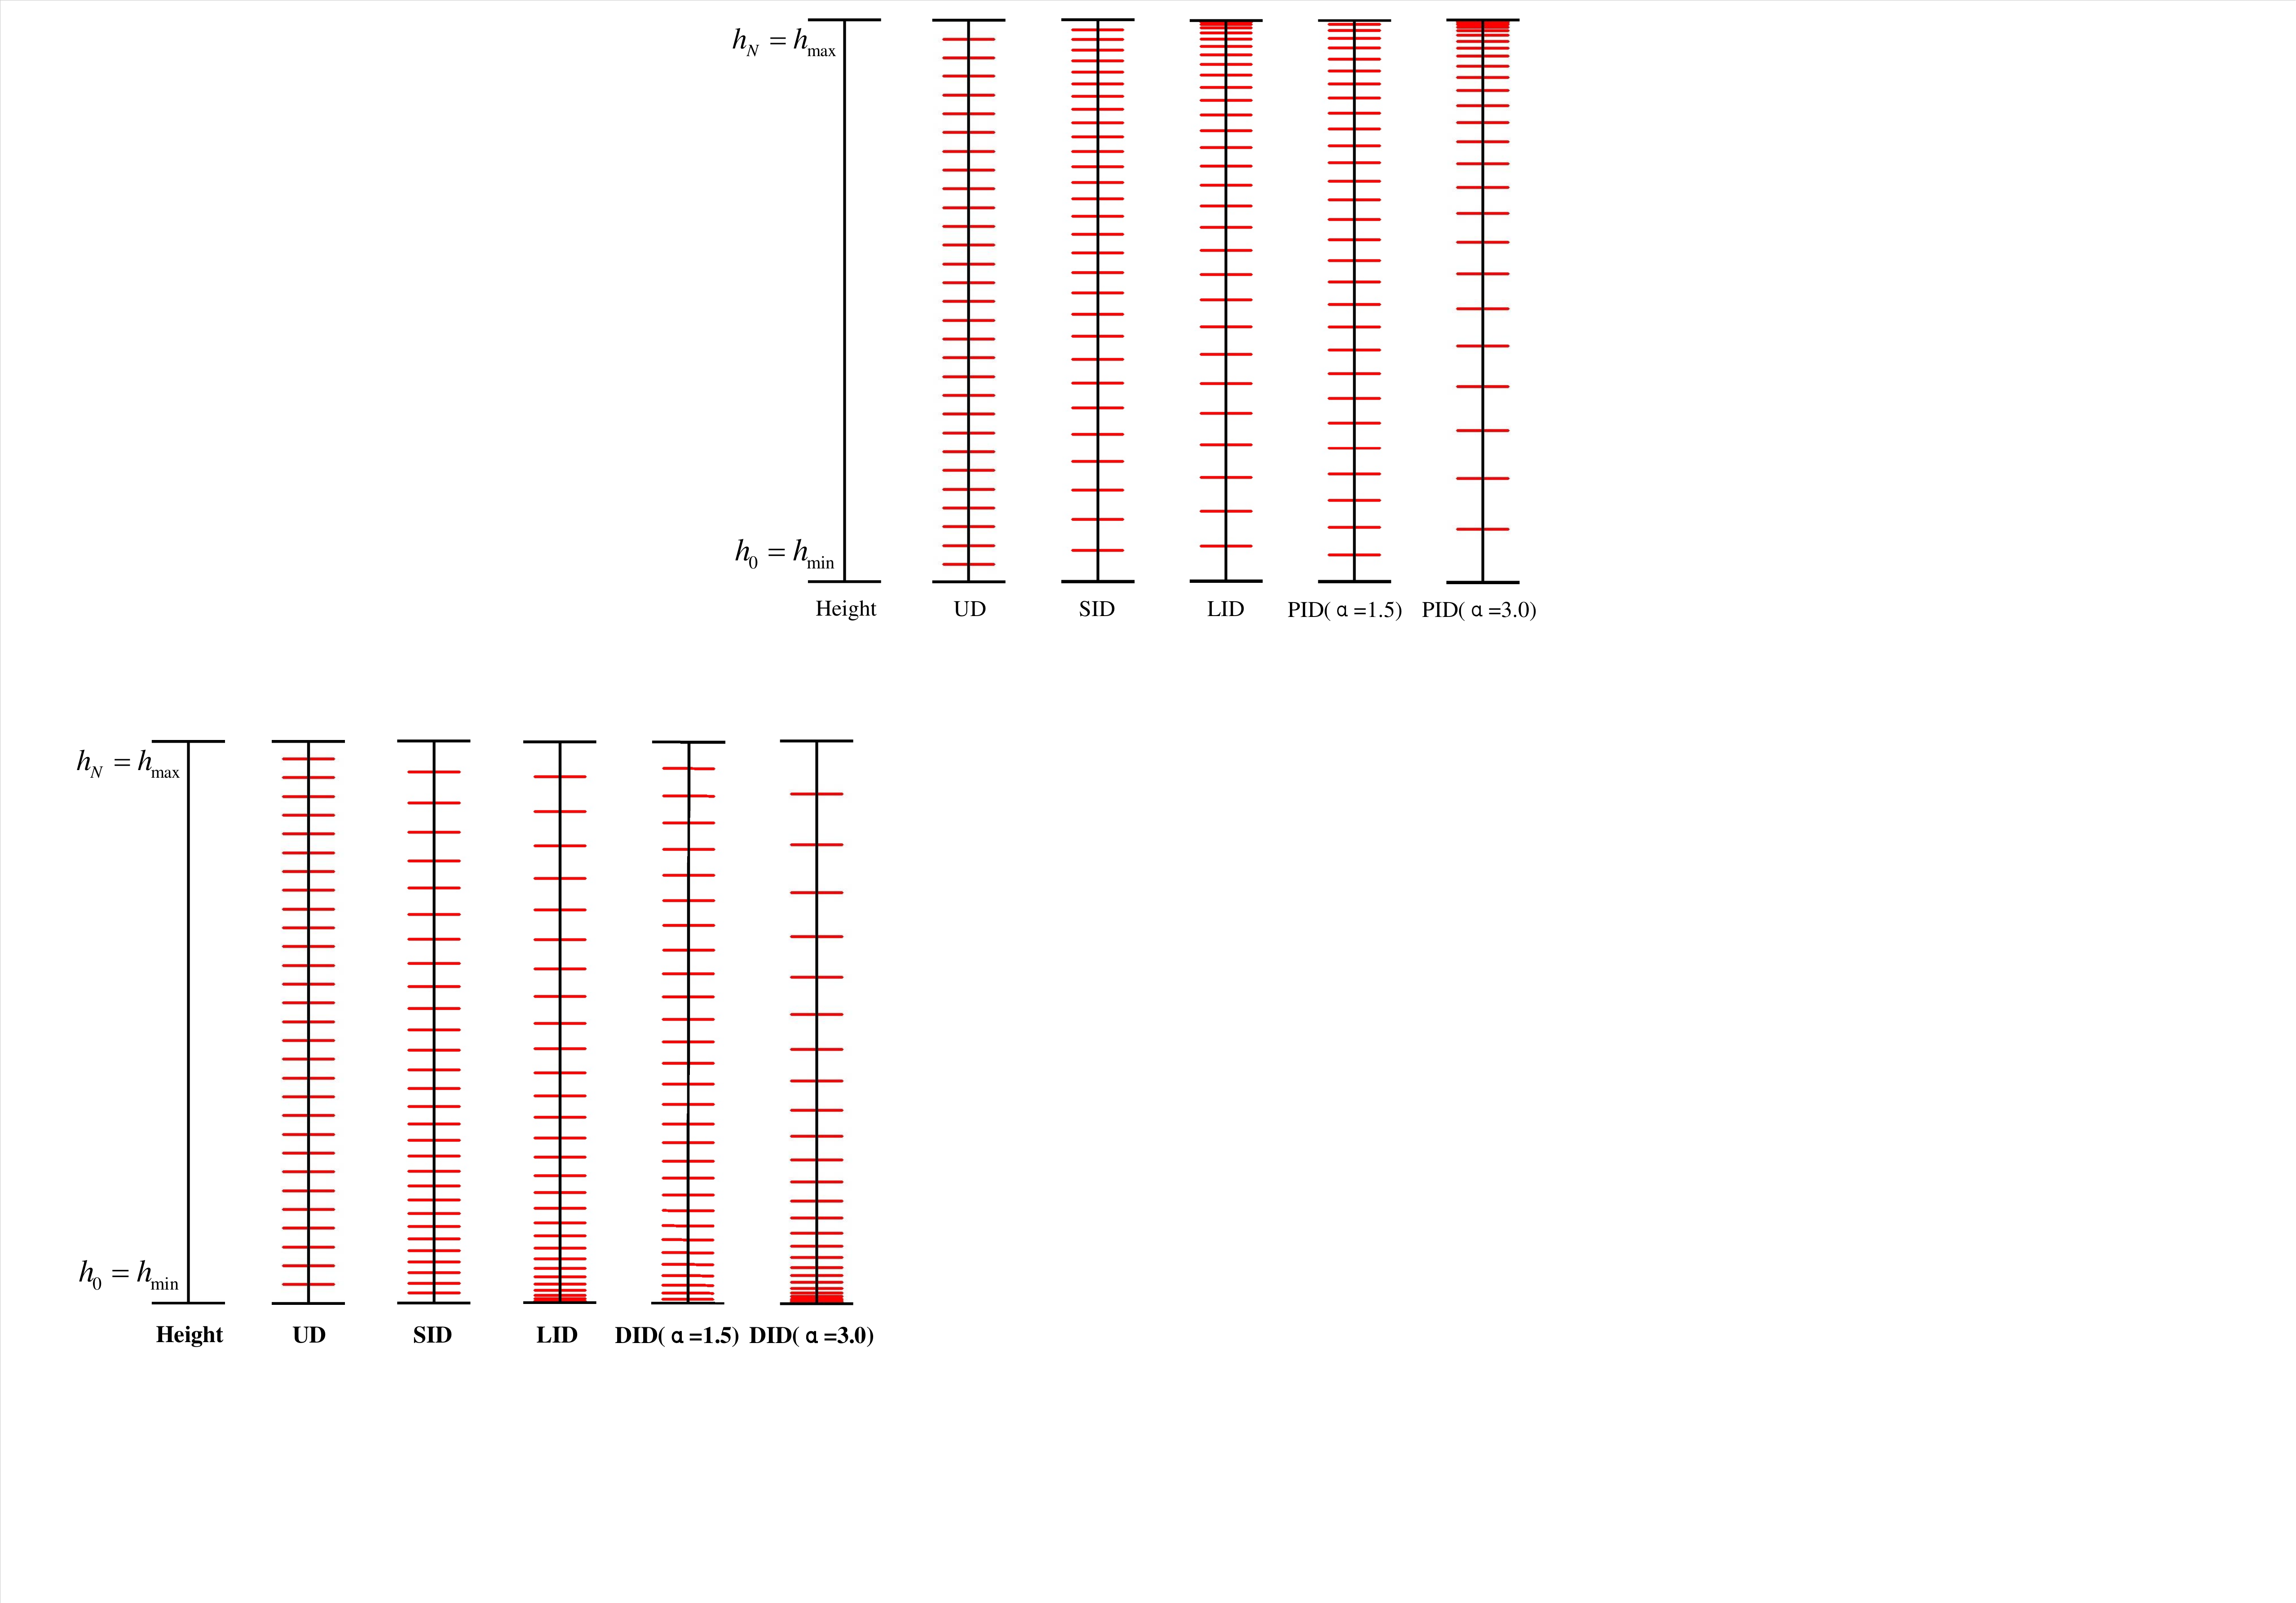}
	\caption{\textbf{Height Discretization Methods.} Height $h_i$ is discretized over a height range $[h_{min}, h_{max}]$ into $N$ discrete bins. From left to right, these are uniform discretization (UD), spacing-increasing discretization (SID), linear-increasing discretization (LID) and the adjustable dynamic-increasing discretization(DID). For the dynamic-increasing discretization (DID) strategy, height bins with large $\alpha$ are more densely distributed when approaching the $h_{min}$ than the small hyper-parameter $\alpha$ conditions.}
\label{fig:discretization}
\end{figure}

\subsection{Results on V2X-Sim Dataset}
To certify the effectiveness of our method in multi-view scenarios, we conduct experiments on V2X-Sim~\cite{li2022v2x} simulation dataset that contains four surround roadside cameras.
As shown in Tab.~\ref{v2x_sim_rebuttal}, our BEVHeight surpass the BEVDepth by more than 10.88\%, 21.15\% on vehicle and cyclist respectively, which verifies the effectiveness of our method.
\input{BEV-Height/latex/table/v2x_sim_rebuttal.tex}

\subsection{Effectiveness on multi depth-based Detectors} We extend our modules on BEVDepth\cite{li2022bevdepth} and BEVDet~\cite{huang2021bevdet} on
 DAIR-V2X-I\cite{yu2022dair} and present the results here. Replacing the depth-based projection in BEVDepth\cite{li2022bevdepth}, our method achieves
a performance increase of 2.19\%, 5.87\%, 4.61\% on vehicle, pedestrian and cyclist. Similarly, our approach surpasses
the origin BEVDet by 8.56\%, 5.35\%, 8.60\% respectively.
\input{BEV-Height/latex/table/bevdet_rebuttal.tex}

% \subsection{More Results}
% \subsubsection{Results on Rope3D Dataset}
\subsection{More Results on DAIR-V2X-I Dataset}
Tab.~\ref{dair} shows the experimental results of deploying our proposed approach on the DAIR-V2X-I\cite{yu2022dair} val set. Under the same configurations (e.g., backbone and BEV resolution), our model outperforms the BEVDepth\cite{li2022bevdepth} baselines by a large marge, which demonstrates the admirable performance of our approach.

% \input{BEV-Height/latex/table/rope3d_het}

% 不同分辨率的泛化性
% 非重要内容，可放在补充材料中(分辨率非主要创新)
\input{BEV-Height/latex/table/dair2_v2.tex}

\input{BEV-Height/latex/fig/visualization_supp}

\subsection{More Visualizations}
In Fig.~\ref{fig:visualization_supp_1} and Fig.~\ref{fig:visualization_supp_2}, we show more visualization results on the DAIR-V2X-I \cite{yu2022dair} dataset. As can be seen from the samples in I/II-(a) clean, our BEVHeight manage to detect objects in middle and long-distances. As for the  extrinsic disturbance cases in  I/II-(b) and I/II-(c),  our method can still guarantee the detection accuracy in terms of cars, pedestrian and cyclist. It can be concluded that our method can significantly improve the accuracy in middle and long-distances and the robustness to extrinsic disturbance.

% \Tao{Can we have some prediction results of height / depth?}
% \Lei{See Sec. ~\ref{sec:distance_error_analysis}, in process}
